# Supplementary material for: GrannGAN: Graph annotation generative adversarial networks
Source: arXiv:2212.00449 source file (2022-12-01)
Supplement: Supplementary file 1 [file supplement.tex]

\newpage

\section{Model details}\label{ann:model}

We describe here the details of our model architecture:

\subsection{General architecture}

The general architecture follows the design outlined in figure \ref{fig:method} in the main paper.
The GrannGAN is composed of two WGAN models, both following the same basic structure.

\subsubsection{Critics}

The critic functions $f$, in both the node-annotation and the edge-annotation models, are message passing networks (MPNNs) with 3 update steps. 
The last step is complemented by node-wise and edge-wise MLP with the following architecture: Linear(64, 128), CELU, Linear(128, 128), CELU, Linear(128, 1).

\subsubsection{Generators}
The generator functions $g$, in both the node-annotation and the edge-annotation models, are MPNNs with 6 update steps.

\subsection{Message passing networks}

The basic architecture of all the MPNNs is described in equations \eqref{eq:edge}-\eqref{eq:nodeaggreg}. 
In the QM9 model, the node update function $\phi_h$ is a sum of small MLPs operating indipendently over the previous hidden state and over the current node update.
In the ZINC model, we have introduced skip connections to both the edge \eqref{eq:edge} and node updates \eqref{eq:nodeaggreg}.

The update functions $\phi$ are all 2 layer, 64-dimensional MLPs with CELU activations.

The random noise variable vectors are $\rvz \in \R^{32}$ sampled from a Gaussian distribution $\rvz \sim \gN(0, \mI)$.

We encode categorical edge and node features as one-hot vectors and use the Straight-Through Gumbel-Softmax approach \cite{jang_categorical_2016} for generating discrete samples with continuous approximation for backpropagation.
Continuous features are produced by a linear layer in the final step of the generator MPNN.

\section{Distribution comparisons}\label{ann:distribs}

We have further explored the bias that enforcing the chemical constraints bring into the distribution modelling.
In figure \ref{fig:graphAF} we compare the length measured in terms of the total number of atoms in the true underlying distribution and in the newly generated instances. 
As the graphs illustrate, there is a large discrepency between these in the GraphAF model.
We hypothesise that by enforcing validity, the model strides away from the underlying distribution to parts of the space that may be easier from the chemical point of view. 

Our model is restricted by the graph skeleton. When the skeletons are sampled directly from the underlying distribution, the distribution of the length of the generated graphs matches the true distribution perfectly by construction. 

\begin{figure}[ht]
\centering
\includegraphics[width=0.4\textwidth]{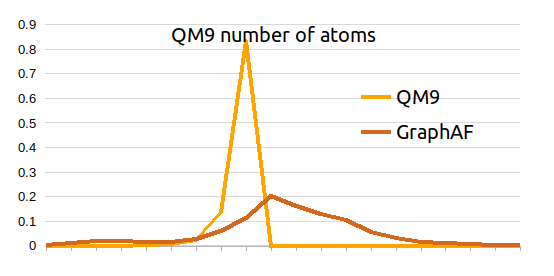}
\includegraphics[width=0.4\textwidth]{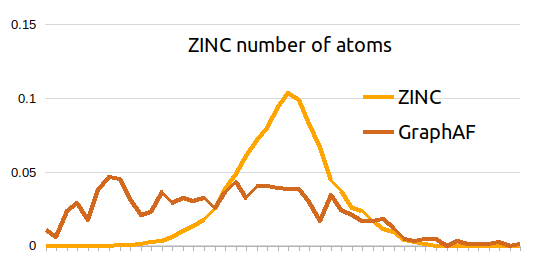}
\caption{GraphAF: empirical distributions of the length (number of nodes) in the real and generated datasets}
\label{fig:graphAF}
\end{figure}
